# Supplementary material for: Atomic-Scale Mechanisms of Li-Ion Transport Mediated by Li10GeP2S12 in Composite Solid Polyethylene Oxide Electrolytes
Source: arXiv:2601.00112 source file (2026-03-28)
Supplement: Supplementary file 1 [file SI.pdf]

# Supporting Information

## Atomic-Scale Mechanisms of Li-Ion Transport Mediated by $\text{Li}_{10}\text{GeP}_2\text{S}_{12}$ in Composite Solid Polyethylene Oxide Electrolytes

*Syed Mustafa Shah*<sup>a,+</sup>, *Musawenkosi K. Ncube*<sup>a,+</sup>, *Mohammed Lemaalem*<sup>a,+</sup>, *Selva Chandrasekaran Selvaraj*<sup>a</sup>, *Naveen K. Dandu*<sup>a</sup>, *Alireza Kondori*<sup>b</sup>, *Gayoon Kim*<sup>b</sup>, *Adel Azaribeni*<sup>b</sup>, *Mohammad Asadi*<sup>b</sup>, *Anh T. Ngo*<sup>a,c,\*</sup>, *Larry A. Curtiss*<sup>c,\*\*</sup>

<sup>a</sup> Department of Chemical Engineering, University of Illinois Chicago, Chicago, IL60608, USA

<sup>b</sup> Department of Chemical and Biological Engineering, Illinois Institute of Technology, Chicago, IL 60616, USA.

<sup>c</sup> Materials Science Division, Argonne National Laboratory, Lemont, IL 60439, USA.

<sup>+</sup> These authors contributed equally to this work.

(\*) anhnngo@uic.edu, (\*\*) curtiss@anl.gov

## 1 Supplementary Information

### 1.1 Molecular Dynamics Simulation Setup

The composite solid polymer electrolyte studied in this work contains  $\text{Li}_{10}\text{GeP}_2\text{S}_{12}$  (LGPS) nanoparticles, methoxy-poly(ethylene oxide)-trimethoxysilane (mPEO-TMS), poly(ethylene oxide) (PEO), and lithium bis(trifluoromethanesulfonyl)imide (LiTFSI), using the molecular weight presented in Table S1. The experimental composition is summarized in Table S2.

The number of molecules  $N$  for each component was calculated from the experimental mass ( $m$ ) and molecular mass ( $M$ ) using:

$$N = \frac{m \times N_A}{M} \quad (1)$$

Table S1: Molecular mass of used components.

| Component         | Molar mass<br>$M$ (g/mol) |
|-------------------|---------------------------|
| LiTFSI            | 287.09                    |
| mPEO-TMS          | 525                       |
| PEO chain         | 2203                      |
| LGPS nanoparticle | 9420.44                   |

Table S2: Experimental composition of the electrolyte.

| Weight Ratio | Element (gram) |          |        |     |
|--------------|----------------|----------|--------|-----|
|              | LGPS           | mPEO-TMS | LiTFSI | PEO |
| 0%           | 0              | 1        | 1.22   | 0.5 |
| 1.3%         | 0.20           | 1        | 1.22   | 0.5 |
| 2%           | 0.031          | 1        | 1.22   | 0.5 |
| 3.20%        | 0.05           | 1        | 1.22   | 0.5 |
| 9%           | 0.148          | 1        | 1.22   | 0.5 |
| 17%          | 0.308          | 1        | 1.22   | 0.5 |
| 21%          | 0.375          | 1        | 1.22   | 0.5 |
| 30%          | 0.64           | 1        | 1.22   | 0.5 |
| 40%          | 1              | 1        | 1.22   | 0.5 |

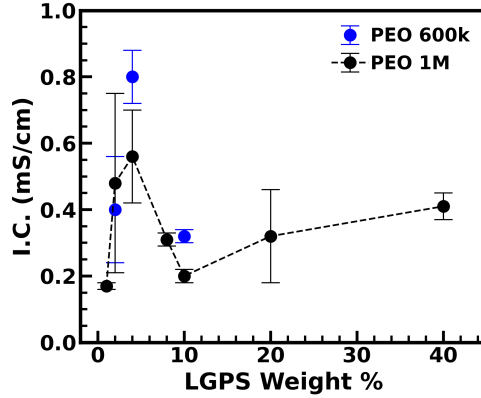

Figure S1: Ionic conductivity as a function of LGPS content in the solid-state electrolyte. Error bars represent the standard deviation from multiple measurements and sample batches. Note that in the paper, the weight percent is defined relative to PEO plus mPEO-TMS, whereas in this plot it is defined relative only to mPEO-TMS.

where  $N_A = 6.022 \times 10^{23} \text{ mol}^{-1}$  is Avogadro's number.

Experimentally, the size of the LGPS nanoparticles in the composite polymer electrolyte is unknown, but the crystallites have a diameter of approximately 17 nm. In the simulations,

due to computational limitations, LGPS was modeled as spherical particles with a radius of 1.2 nm. Then, the number of particles used in the MD simulations was adjusted to conserve the experimental mass ratios.

The Universal Force Field (UFF) was used for mPEO-TMS and LGPS, while the OPLS-AA force field was applied to  $\text{Li}^+$ ,  $\text{TFSI}^-$ , and PEO chains. A Lennard-Jones and Coulombic cut-off radius of  $r_{\text{cut}} = 14 \text{ \AA}$  was applied. Long-range electrostatics were computed using the PPPM solver with an accuracy of  $10^{-4}$  [1]. Initial configurations were generated using the Moltemplate package [2]. Molecules were randomly placed in an oversized cubic cell and energy-minimized via iterative coordinate adjustments [3]. The stopping tolerances for minimization were  $E_{\text{stop}} = 10^{-7}$  (unitless, change in energy per iteration normalized to total energy) and  $F_{\text{stop}} = 10^{-8} \text{ kcal mol}^{-1} \text{ \AA}^{-1}$ . Equilibration and production followed a four-step protocol: agitation using a Langevin thermostat at 900 K for 1 ns followed by a Nosé–Hoover thermostat at 900 K; temperature ramping from 900 K to 300 K at  $P = 500 \text{ bar}$  over 3 ns in the NPT ensemble; pressure ramping from  $P = 500 \text{ bar}$  to  $P = 1 \text{ bar}$  at  $T = 300 \text{ K}$  over 3 ns; and a final equilibration under the NPT ensemble at  $T = 300 \text{ K}$  and  $P = 1 \text{ bar}$  for 10 ns using a Berendsen barostat [4]. Production runs were then conducted in the NVT ensemble at  $T = 300 \text{ K}$  using a Nosé–Hoover thermostat for transport property analysis. The simulation time step was  $\Delta t = 1 \text{ fs}$  for all stages.

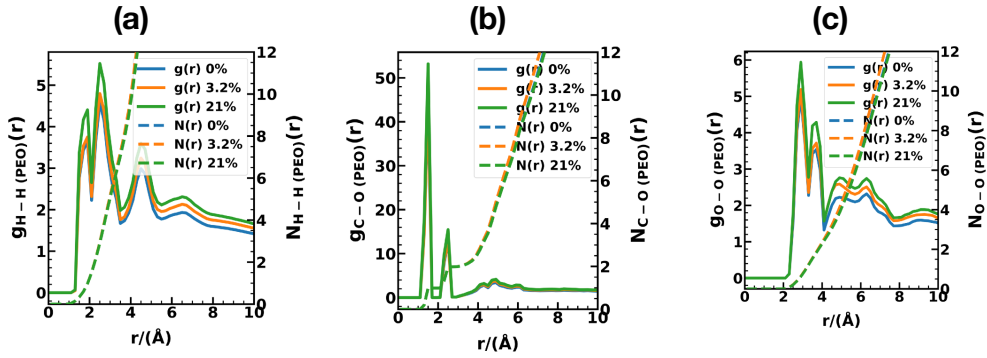

Figure S2: RDF and  $N(r)$  for selected atomic pairs (H–H, C–O, and O–O) in poly(ethylene oxide) (PEO).

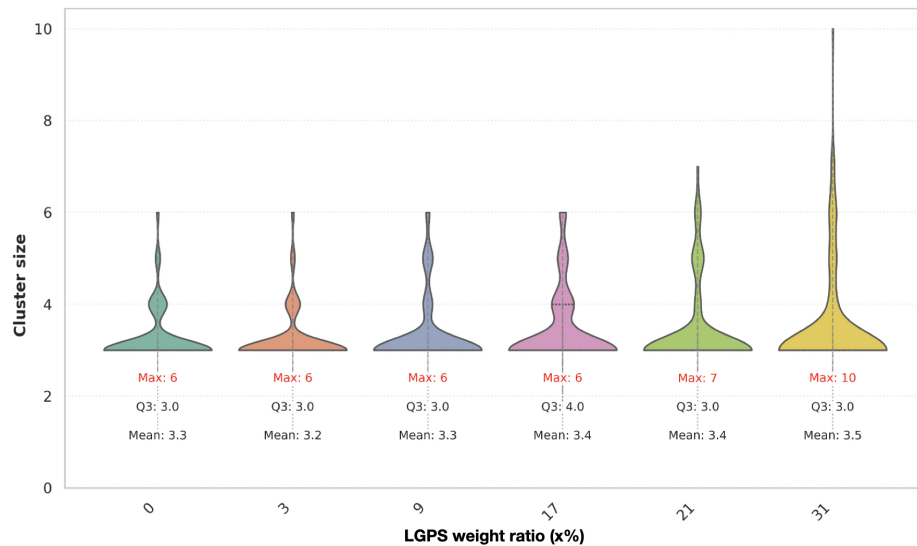

Figure S3: Li ion formed clusters within the composite polymer electrolyte (CPE) for different LGPS weight ratio.

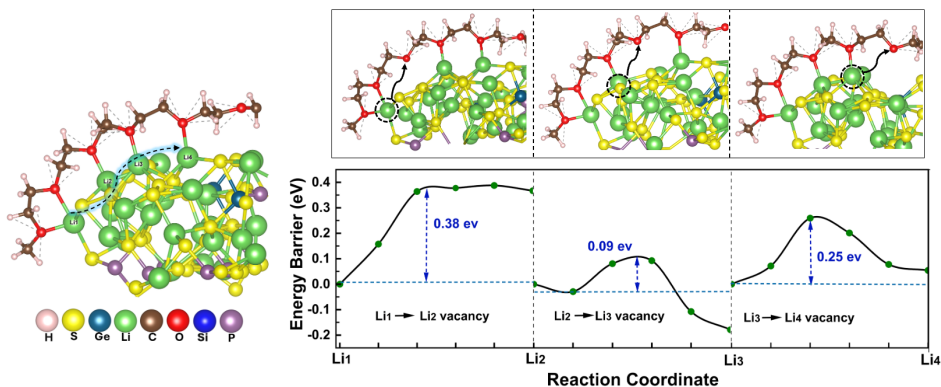

Figure S4: The effect of modifying the atomic composition and bonding on the mPEO-TMS|LGSP interface to enhance Li-ion transport.

## References

- [1] W. McDoniel, M. Höhnerbach, R. Canales, A. E. Ismail, P. Bientinesi, LAMMPS' PPPM long-range solver for the second generation xeon phi, in: International Conference on High Performance Computing, Springer, 2017, pp. 61–78.
- [2] A. Jewett, Moltemplate manual, University of California, Santa Barbara Shea Lab (August 2015) (2020).

- [3] J. Guenole, W. G. Noehring, A. Vaid, F. Houle, Z. Xie, A. Prakash, E. Bitzek, Assessment and optimization of the fast inertial relaxation engine (FIRE) for energy minimization in atomistic simulations and its implementation in LAMMPS, *Computational Materials Science* 175 (2020) 109584.
- [4] T. J. Barrett, M. L. Minus, Thermostat, barostat, and damping parameter impact on the tensile behavior of graphene, Available at SSRN 4289377 (2023).
